# Supplementary material for: Scalable Online Exploration via Coverability
Source: arXiv:2403.06571 source file (2024-06-04)
Supplement: Supplementary file 2 [file appendix_additional_properties-arxiv.tex]

\subsection{Additional Results}

More generally, for any $q\in[1,\infty)$, one can consider the $L_q$-Coverability
objective given by
\[
\qCovM(p) = \sup_{\pi\in\Pi}\sup_{(x,a)\in\cX\times\cA}\prn*{\En^{\sM,\pi}\brk*{\prn*{\frac{d^{\sM,\pi}_h(x,a)}{d_h^{\sM,p}(x,a)+\veps\cdot{}d_h^{\sM,\pi}(x,a)}}^{q}}}^{1/q}
  \mathand \qCovOptM = \inf_{p\in\Delta(\Pi)}\qCovM(p),
\]
For $\veps>0$, we can upper bound this quantity by passing to \mainobj:
  \begin{align}
(\qCovOptM)^q \leq \frac{\CovOptM}{\veps^{q-1}} \leq \frac{\CinfhM}{\veps^{q-1}},
  \end{align}
  so that $\qCovOptM \leq (\CinfhM)^{1/q}/\veps^{1-1/q}$. Interestingly, a straightforward generalization of
\cref{prop:linf_impossibility} shows this naive upper bound is
(nearly) tight.
\begin{restatable}{proposition}{lqimpossibility}
  \label{prop:lq_impossibility}
  Let $q>1$ be given. For any $\delta>0$, there exists an MDP $M$ and policy class
  $\Pi\subset\PiRNS$ with horizon $H=1$ such that $\CinfhM\leq{}2+\frac{1}{\delta{}q}$ (and hence
  $\CovOptM\leq{}2+\frac{1}{\delta{}q}$ as well), yet for all
  $\veps>0$,
  \begin{align}
    \label{eq:lq_impossibility}
  \qCovOptM
  \geq \frac{1}{4\veps^{1-\frac{1}{q}-\delta}}.
  \end{align}
 and in particular $\cov_{q;h,0}=\infty$.
\end{restatable}
